# Supplementary material for: InfiniteTalk: Audio-driven Video Generation for Sparse-Frame Video Dubbing
Source: arXiv:2508.14033 source file (2025-08-19)
Supplement: Supplementary file 1 [file x_appendix.tex]

\appendix
% \section{Appendix}
